# Supplementary material for: Multimodal Fusion of RGB and Complementary Modalities for Semantic Segmentation
Source: arXiv:2610.17800 source file (2026-10-13)
Supplement: Supplementary file 1 [file appendix.tex]

% Source archive only: all previously active appendix material has been integrated into
% sections/04_experiments.tex and sections/06_discussion.tex. Do not input this file.
% Original lines are preserved below as comments; deferred alternatives remain disabled.

% \section{Supplementary Experimental Details}
% \subsection{Dataset Details}
% \label{app:datasetdetails}
% \begin{wraptable}{r}{0.44\textwidth}
% \centering
% \compacttablefont
% \caption[Common configuration parameters]{Common configuration hyperparameters.}
% \fitbox{%
% \begin{tabular}{ll}
% \toprule
% \textbf{Parameter} & \textbf{Value} \\
% \midrule
% Background & 255 \\
% Learning Rate (LR) Power & 0.9 \\
% Momentum & 0.9 \\
% Weight Decay & 0.01 \\
% Batch Size & 2 \\
% Number of Workers & 2 \\
% Train Scale Array & {[0.5, 0.75, 1, 1.25, 1.5, 1.75]} \\
% Warm-up Epochs & 10 \\
% Fix Bias & True \\
% Batch Norm Epsilon & 1e-3 \\
% Batch Norm Momentum & 0.1 \\
% Evaluation Iteration & 25 \\
% Evaluation Stride Rate & 2/3 \\
% Evaluation Scale Array & {[1]} \\
% Evaluation Flip & False \\
% \bottomrule
% \end{tabular}%
% }
% \label{tab:common_config}
% \end{wraptable}
% 
% An overview of the datasets used in our experiments is provided in Tab.~\ref{tab:dataset_overview}. The details are introduced below:
% \textbf{RGB-T MFNet}~\cite{ha2017mfnet} is a driving-scene dataset with 1,569 aligned RGB-thermal pairs across 8 semantic classes. It provides 784/392/392 images for training, validation, and testing, respectively, covering both daytime and nighttime conditions.  
% 
% \textbf{RGB-L KITTI-360}~\cite{liao2022kitti} is a suburban
% driving dataset, providing 49,004 training and 12,276 validation images with a resolution of $1408 \times 376$. Following the Cityscapes dataset~\cite{cordts2016cityscapes}, it defines 19 semantic classes.
% 
% 
% \textbf{RGB-X DELIVER}~\cite{zhang2023delivering} is a large-scale synthetic benchmark built in the CARLA simulator, supporting multi-modal segmentation across RGB, depth, event, and LiDAR streams. It contains over 47k annotated frames from six camera views under diverse conditions, including challenging weather (fog, rain, night) and five sensor degradation types (e.g., motion blur, exposure imbalance, LiDAR jitter). The dataset defines 25 semantic classes covering urban elements such as vehicles, roads, pedestrians, and vegetation. 
% 
% \textbf{RGB-E DDD17}~\cite{Binas2017DDD17ED} includes over 12 hours of driving data collected with a DAVIS346B sensor, providing event streams and grayscale images at $200 \times 346$ resolution. We generate pseudo-labels using EV-SegNet~\cite{alonso2019ev}, resulting in 5 semantic classes and splits of 15,950/3,890 samples.  
% 
% \textbf{RGB-E DSEC}~\cite{gehrig2021dsec} contains over 10k RGB-event frames with 11 categories, captured from stereo cameras in urban and rural environments. We follow~\cite{xie2024eisnet} for preprocessing and dataset splits (8082/2809 for training/testing).  
% 
% \textbf{RGB-P MCubeS}~\cite{liang2022multimodal} consists of 500 samples with aligned RGB, NIR, and polarization cues (DoLP, AoLP), annotated with 20 material categories. The dataset is split into 302/96/102 for training, validation, and testing.  
% 
% 
% \textbf{RGB-P ZJU}~\cite{xiang2021polarization} is a polarization semantic segmentation dataset collected in outdoor scenes. 
% Each sample contains four polarized RGB images at $0^\circ$, $45^\circ$, $90^\circ$, and $135^\circ$, from which AoLP and DoLP are derived using Stokes parameters. It provides 344 training and 50 validation samples across 8 semantic classes, with image resolution of $1224 \times 1024$.
% 
% 
% 
% \textbf{RGB-LF UrbanLF}~\cite{sheng2022urbanlf} is a light-field dataset for urban-scene segmentation, including both real (580/80/164) and synthetic (172/28/50) subsets, each with 14 semantic classes. Central-view annotations are used for supervision.
% 
% \wrapfinish
% 
% \subsection{Common Configuration Parameters}
% \label{app:impdetails}
% 
% 
% \subsection{Evaluation Metrics}
%  \label{sec:metrics}
% 
%  
% 
%  \subsection{Intersection over Union (IoU):}
%  IoU quantifies the overlap between the predicted and ground truth segmentation masks for each class. It is defined as:
%  \begin{equation}
%  \text{IoU}_c = \frac{|A_c \cap B_c|}{|A_c \cup B_c|},
%  \end{equation}
%  where $A_c$ and $B_c$ denote the predicted and ground truth pixels for class $c$, respectively. A higher IoU indicates better boundary delineation and region matching.
% 
%  \subsection{Mean IoU (mIoU):}
%  The primary evaluation metric is mIoU, which averages IoU scores across all classes, ensuring a balanced evaluation regardless of class frequency. Formally,
%  \begin{equation}
%  \text{mIoU} = \frac{1}{C} \sum_{c=1}^{C} \frac{|A_c \cap B_c|}{|A_c \cup B_c|},
%  \end{equation}
%  where $C$ is the total number of classes. This metric is particularly valuable in datasets with diverse categories, such as autonomous driving, where rare classes (e.g., pedestrians) must be treated with equal importance as dominant ones (e.g., road).
% 
% \subsection{Frequency Weighted IoU (FWIoU):}
% FWIoU incorporates class frequency into the IoU computation, emphasizing the performance on common classes. It is defined as:
% \begin{equation}
% \text{FWIoU} = \sum_{c=1}^{C} \frac{n_c}{N} \cdot \frac{|A_c \cap B_c|}{|A_c \cup B_c|},
% \end{equation}
% where $n_c$ is the number of ground truth pixels for class $c$ and $N$ is the total number of pixels. This metric highlights model performance under class imbalance, which is typical in road-scene datasets.
% 
% \subsection{Pixel Accuracy (PA):}
% Pixel accuracy reflects the ratio of correctly classified pixels over the entire dataset:
% \begin{equation}
% \text{PA} = \frac{\text{Correctly Classified Pixels}}{\text{Total Number of Pixels}}.
% \end{equation}
% While intuitive, this metric may overestimate performance if dominant classes occupy large portions of the image.
% 
% \subsection{Mean Pixel Accuracy (mPA):}
% mPA evaluates pixel-level classification accuracy within each class, averaged across classes:
% {\fontsize{9bp}{11bp}\selectfont
% \begin{equation}
% \text{mPA} = \frac{1}{C} \sum_{c=1}^{C} \frac{\text{Correctly Classified Pixels in Class } c}{\text{Total Pixels in Class } c}.
% \end{equation}
% }
% 
% This ensures that minority classes are not overshadowed by dominant ones, complementing PA and mIoU for a fairer evaluation.
% 
%  \subsection{Computational Efficiency Metrics:}
%  To assess efficiency, we additionally report the computational cost of each model, including floating-point operations (FLOPs), number of parameters, and inference speed measured in frames per second (FPS). FLOPs estimate the theoretical workload of a forward pass, parameter count reflects model size and memory footprint, and FPS measures practical deployment speed under fixed input resolution.
% 
%  \noindent
%  By jointly analyzing these metrics, we achieve a comprehensive evaluation of both segmentation quality and computational efficiency.
% 
% \Needspace{120pt}
% \subsection{Backbone Comparison}
% % Pending numerical-version audit: MCubeS 52.5 here versus 52.22 in the quantitative table.
% \begin{wraptable}{r}{0.36\textwidth}
% \centering
% \compacttablefont
% \caption{Backbone comparison in mIoU(\%).}
% \label{tab:backbone_ablation}
% \fitbox{%
% \begin{tabular}{lcc}
% \toprule
% Backbone & MCubeS & MFNet \\
% \midrule
% MiT-B2 & 50.1 & 74.1\\
% MiT-B4 & 52.5 & 76.9\\
% \bottomrule
% \end{tabular}%
% }
% \end{wraptable}
% 
% To verify that our performance gains are not driven by backbone scaling, we additionally evaluate both MiT-B2 and MiT-B4 on the MCubeS and MFNet dataset (Tab.~\ref{tab:backbone_ablation}), where MiT-B4 improves overall accuracy as expected, while the relative advantage of our method remains consistent across backbone choices.
% 
% 
% \wrapfinish
% 
% \subsection{Per-class Results}
% \label{app:perclass}
% %\subsection{Further Results Analysis}
% 
% 
%  %\subsubsection{Results on RGB-Thermal Datasets}
%  \begin{wraptable}{r}{0.46\textwidth}
% \centering
% \compacttablefont
% \caption[Per-class results on MFNet~\cite{ha2017mfnet}]{Per-class IoU and overall metrics comparison between the baseline~\cite{cao2024embracing} and our proposed model on the MFNet dataset~\cite{ha2017mfnet} after 60 epochs of training.}
% \label{tab:mfnet_classwise}
% \renewcommand{\arraystretch}{1.05}
% \setlength{\tabcolsep}{3pt}
% \fitbox{%
% \begin{tabular}{l|cc}
% \toprule
% \textbf{Class IoU (\%)} & \textbf{Baseline~\cite{cao2024embracing}} & \textbf{Our Model} \\
% \midrule
% 1. Car         & 93.97  & 97.31 \\
% 2. Person      & 87.66  & 88.95 \\
% 3. Bike        & 81.26  & 86.62 \\
% 4. Curve       & 90.50  & 93.14 \\
% 5. Car Stop    & 32.73  & 67.66 \\
% 6. Guardrail   & 8.06   & 28.96 \\
% 7. Color Cone  & 63.14  & 60.97 \\
% 8. Bump        & 80.40  & 90.27 \\
% \midrule
% Mean IoU       & 67.21  & \textbf{76.74} \\
% Freq IoU       & 87.65  & \textbf{92.33} \\
% Mean Pixel Acc.& 77.29  & \textbf{89.53} \\
% Pixel Accuracy & 92.87  & \textbf{95.74} \\
% \bottomrule
% \end{tabular}%
% }
% 
% \end{wraptable}
% 
% \subsection{MFNet (60-epoch setting).}
% In addition to the overall comparison reported in the main paper, we provide a per-class analysis on MFNet~\cite{ha2017mfnet} in Table~\ref{tab:mfnet_classwise}. 
% Our model consistently outperforms the baseline~\cite{cao2024embracing} across most categories. 
% Notable gains are observed on challenging classes such as \textit{Car Stop} (+34.93\%) and \textit{Guardrail} (+20.90\%), demonstrating improved detection of small or subtle structures. For common categories like \textit{Car}, \textit{Bike}, and \textit{Bump}, we also observe clear improvements, indicating better boundary handling and stronger representations of dominant objects. The only minor drop appears in \textit{Color Cone}, likely due to limited samples. 
% Overall, these results confirm the effectiveness of our framework in enhancing both frequent and rare categories, leading to higher mIoU and pixel-level accuracy.
% 
% 
% 
%  %\subsubsection{Results on RGB-Event Datasets}
%  %\subsection{DSEC.}
%  %In addition to the overall performance comparison, we provide a detailed per-class analysis on the DSEC dataset~\cite{gehrig2021dsec}. As reported in Table~\ref{tab:dsec_classwise}, our model achieves consistent improvements over the baseline~\cite{cao2024embracing} in most categories. Notably, \textit{Fence} and \textit{Building} show clear gains of +2.04\% and +1.77\% IoU, reflecting better handling of fine structures and distant regions. Foreground categories such as \textit{Car}, \textit{Road}, and \textit{Wall} also benefit from stable improvements, while large-area classes like \textit{Vegetation} and \textit{Sidewalk} are well preserved. Although \textit{Person} shows a marginal decrease of 0.40\%, the overall segmentation quality remains unaffected, and most dominant categories such as \textit{Pole} maintain their performance. These results confirm that our fusion strategy enhances both fine-grained boundaries and region-dense predictions, leading to improved semantic consistency across the dataset.
% 
%  %\begin{table}[htbp]
%  %\centering
%  %\renewcommand{\arraystretch}{1.2}
%  %\setlength{\tabcolsep}{8pt}
%  %\begin{tabular}{l|cc}
%  %\toprule
% % \textbf{Class IoU (\%)} & \textbf{Baseline~\cite{cao2024embracing}} & \textbf{Our Model} \\
% % \midrule
% % Background     & 91.00  & 91.34 \\
% % Building       & 34.70  & 36.47 \\
% % Fence          & 66.38  & 68.42 \\
% % Person         & 63.59  & 63.19 \\
% % Pole           & 96.56  & 96.56 \\
% % Road           & 81.41  & 81.52 \\
% % Sidewalk       & 94.52  & 94.54 \\
% % Vegetation     & 92.42  & 92.52 \\
% % Car            & 47.36  & 47.85 \\
% % Wall           & 74.70  & 75.26 \\
% % \midrule
% % Mean IoU           & 74.26  & \textbf{74.77} \\
% % Frequency IoU      & 91.81  & \textbf{91.92} \\
% % Mean Pixel Acc.    & 81.16  & \textbf{81.70} \\
% % Pixel Accuracy     & 95.52  & \textbf{95.60} \\
% % \bottomrule
% % \end{tabular}
% % \caption[Per-class results on DSEC~\cite{gehrig2021dsec}]{
% % Per-class IoU and overall metrics on the DSEC dataset~\cite{gehrig2021dsec}.}
% % \label{tab:dsec_classwise}
% % \end{table}
% 
% \wrapfinish
% 
% \begin{wraptable}{r}{0.46\textwidth}
% \centering
% \compacttablefont
% \caption[Per-class results on DDD17~\cite{Binas2017DDD17ED}]{
% Per-class IoU and overall metrics on the DDD17 dataset~\cite{Binas2017DDD17ED} with models trained for 40 epochs. 
% }
% \label{tab:ddd17_classwise}
% \renewcommand{\arraystretch}{1.05}
% \setlength{\tabcolsep}{3pt}
% \fitbox{%
% \begin{tabular}{l|cc}
% \toprule
% \textbf{Class IoU (\%)} & \textbf{Baseline~\cite{cao2024embracing}} & \textbf{Our Model} \\
% \midrule
% Flat          & 96.51  & 96.73 \\
% Object        & 40.54  & 41.80 \\
% Vegetation    & 81.87  & 82.94 \\
% Human         & 75.53  & 77.59 \\
% Vehicle       & 90.11  & 90.20 \\
% \midrule
% Mean IoU           & 76.91  & \textbf{77.85} \\
% Frequency IoU      & 94.22  & \textbf{94.54} \\
% Mean Pixel Acc.    & 82.78  & \textbf{84.47} \\
% Pixel Accuracy     & 96.91  & \textbf{97.10} \\
% \bottomrule
% \end{tabular}%
% }
% 
% \end{wraptable}
% 
% \subsection{DDD17.}
% We further provide a per-class analysis on the DDD17 dataset~\cite{Binas2017DDD17ED}. As shown in Table~\ref{tab:ddd17_classwise}, our model consistently outperforms the baseline~\cite{cao2024embracing} across all five semantic categories. In particular, \textit{Human} and \textit{Vegetation} exhibit notable gains of +2.06\% and +1.07\% IoU, reflecting improved representation of dynamic and detailed structures. Meanwhile, \textit{Object} and \textit{Vehicle} achieve moderate improvements, while \textit{Flat} maintains a very high IoU above 96\%. 
% These results indicate that our fusion strategy not only strengthens predictions for small or fine-grained categories but also preserves the accuracy of dominant regions, contributing to the overall performance gain on this challenging large-scale driving dataset.
% 
% 
% 
% 
% % \subsubsection{Results on RGB-Depth Datasets}
% % \subsection{DELIVER-Depth.}
%  
% % Table~\ref{tab:deliver_classwise} further shows consistent per-class improvements, with large gains on \textit{Bridge} (+18.50\%), \textit{Wall} (+6.61\%), and \textit{Pole} (+4.33\%), as well as stable increases for common traffic-related categories such as \textit{Road}, \textit{Cars}, and \textit{Bus}. Background classes like \textit{Building}, \textit{Vegetation}, and \textit{Sky} also benefit from 2--3\% higher IoU, while smaller categories such as \textit{Traffic Light} and \textit{Pedestrian} see modest but positive gains. Overall, these results demonstrate that our design improves both global metrics and per-class predictions across dominant and detail-sensitive regions.
% 
% % \begin{table}[t!]
% % \centering
% % \renewcommand{\arraystretch}{1.2}
% %% \setlength{\tabcolsep}{8pt}
% % \begin{tabular}{l|cc}
% % \toprule
% % \textbf{Class IoU (\%)} & \textbf{Baseline~\cite{cao2024embracing}} & \textbf{Our Model} \\
% % \midrule
% % Building     & 78.56  & 80.86 \\
% % Fence        & 44.24  & 47.44 \\
% % Pedestrian   & 41.01  & 43.77 \\
% % Pole         & 34.79  & 39.12 \\
% % Road         & 95.56  & 97.54 \\
% % Sidewalk     & 79.58  & 82.14 \\
% % Vegetation   & 71.40  & 73.82 \\
% % Cars         & 77.56  & 79.11 \\
% % Wall         & 69.91  & 76.52 \\
% %% Sky          & 94.83  & 96.77 \\
% % Bridge       & 52.81  & 71.31 \\
% % Traffic Light& 39.09  & 42.43 \\
% % Bus          & 76.32  & 79.72 \\
% % Truck        & 80.38  & 81.71 \\
% % \midrule
% % Mean IoU           & 60.55  & \textbf{64.18} \\
% % Frequency IoU      & 86.53  & \textbf{86.72} \\
% % Mean Pixel Acc.    & 69.73  & \textbf{71.08} \\
% % Pixel Accuracy     & 92.36  & \textbf{93.68} \\
% % \bottomrule
% % \end{tabular}
% % \caption[Per-class results on DELIVER-Depth~\cite{zhang2023delivering}]{
% % Per-class IoU and overall metrics comparison between the baseline~\cite{cao2024embracing} and our proposed model on the DELIVER-Depth dataset~\cite{zhang2023delivering}. 
% % All models are trained for 60 epochs.}
% %% \label{tab:deliver_classwise}
% % \end{table}
% 
% \wrapfinish
% 
% \subsection{Impact Statement}
% This paper aims to advance foundational research in the field of multimodal semantic segmentation by providing diverse complementary sensors (e.g., thermal, LiDAR, event) to enhance the RGB images.
% Our work may contribute to safety-critical applications of autonomous driving and robotic perception by ensuring a reliable and robust performance under extreme conditions inlcuding low illumination, adverse weather and severe motion blur. 
% This has the potential to reduce acceident rates and enhance the safety of intelligent systems. 
% Additionally, we acknowledge that deploying transformer-based multi-sensor systems introduces increased computational overhead, emphasizing the importance of future research into lightweight, energy-efficient AI solutions to minimize environmental impact.
% 
% % Historical commented alternatives retained for review; do not enable duplicate labels.
% % \subsection{Qualitative Analysis}
% 
% % \begin{figure*}[t!]
% %   \centering
% %   \includegraphics[width=\linewidth, trim=3cm 2cm 11cm 1cm, clip]{figures/qualitative.pdf}
% %   \caption{Qualitative results across multiple modalities. Our model consistently produces sharper boundaries and more accurate object recognition under challenging conditions.}
% %   \label{fig:qualitative}
% % \end{figure*}
% 
% % In Fig.~\ref{fig:qualitative}, we present qualitative comparisons on five representative datasets: MFNet~\cite{ha2017mfnet} (RGB-Thermal), KITTI-360~\cite{liao2022kitti} (RGB-LiDAR), DSEC~\cite{gehrig2021dsec} (RGB-Event), ZJU-RGBP~\cite{xiang2021polarization} (RGB-Polarization), and UrbanLF-real~\cite{sheng2022urbanlf} (RGB-LightField). On MFNet, our method more clearly distinguishes pedestrians—particularly small and distant ones—that the baseline often fails to separate from the background. On KITTI-360, it delineates roadside trees with sharper boundaries and smoother transitions between vegetation and surrounding regions. On DSEC, our model suppresses spurious responses in the background sky, yielding more stable predictions under fast-motion conditions. On ZJU-RGBP, improvements are evident around reflective surfaces, where pedestrians and vehicle windows are predicted with higher accuracy and fewer artifacts. On UrbanLF-real, our approach provides more consistent segmentation of riders, pedestrians, and background elements, maintaining coherent parsing even under occlusion. Across all benchmarks, these qualitative visualizations show that our fusion strategy consistently produces more reliable results, underscoring its superiority across diverse sensing scenarios.
% %\begin{table}[htbp]
% %\centering
% %\resizebox{\textwidth}{!}{ 
% %\renewcommand{\arraystretch}{1.2}
% %\setlength{\tabcolsep}{5pt}
% %\begin{tabular}{l|c|c|cc}
% %\toprule
% %\textbf{Method} & \textbf{Venue} & \textbf{Modality} & \textbf{Mean IoU (\%)}~$\uparrow$ & \textbf{Pixel Acc (\%)}~$\uparrow$ \\
% %\midrule
% %\multicolumn{5}{c}{\textbf{RGB+Event Methods}} \\
% %\midrule
% %Baseline~\cite{cao2024embracing} & ECCV'24 & RGB+Event & 76.91 & 96.91 \\
% %Our Model & - & RGB+Event & \textbf{77.85} & \textbf{97.10} \\
% %\midrule
% %EFNet~\cite{zhang2025exploiting} & ICMR'25 & RGB+Event & 77.36 & 96.36 \\
% %Hybrid-Segmentation~\cite{li2025efficient} & AAAI'25 & RGB+Event & 67.31 & 95.07 \\
% %EISNet~\cite{xie2024eisnet} & TMM'24 & RGB+Event & 75.03 & 96.04 \\
% %HALSIE~\cite{das2024halsie} & WACV'24 & RGB+Event & 60.66 & 92.50 \\
% %SpikingEDN~\cite{zhang2024accurate} & TNNLS'24 & RGB+Event & 53.15 & - \\
% %CMNeXt~\cite{zhang2023delivering} & CVPR'23 & RGB+Event & 72.67 & 95.74 \\
% %CMX~\cite{zhang2023cmx} & TITS'23 & RGB+Event & 71.88 & 95.64 \\
% %EV-Transfer~\cite{messikommer2022bridging} & RA-L'22 & RGB+Event & 14.91 & 47.37 \\
% %EDCNet-S2D~\cite{zhang2021exploring} & TITS'21 & RGB+Event & 61.99 & 93.80 \\
% %\midrule
% %\multicolumn{5}{c}{\textbf{Event-only Methods}} \\
% %\midrule
% %KWYAF~\cite{li2025know} & AAAI'25 & Event & 57.69 & 90.04 \\
% %ESEG-B~\cite{zhao2025eseg} & AAAI'25 & Event & 57.01 & 89.64 \\
% %ESEG-L~\cite{zhao2025eseg} & AAAI'25 & Event & 59.97 & 90.68 \\
% %OpenESS~\cite{kong2024openess} & CVPR'24 & Event & 63.00 & 91.05 \\
% %EvSegFormer~\cite{jia2023event} & TIP'23 & Event & 54.41 & 94.72 \\
% %ESS-Sup*~\cite{sun2022ess} & ECCV'22 & Event & 61.37 & 91.08 \\
% %ESS-Sup~\cite{sun2022ess} & ECCV'22 & Event & 56.67 & 89.12 \\
% %ESS~\cite{sun2022ess} & ECCV'22 & Event & 53.09 & 88.43 \\
% %EvDistill~\cite{wang2021evdistill} & CVPR'21 & Event & 58.02 & - \\
% %DTL~\cite{wang2021dual} & ICCV'21 & Event & 58.80 & - \\
% %SegFormer~\cite{xie2021segformer} & NIPS'20 & Event & 52.76 & 89.34 \\
% %Vid2E~\cite{gehrig2020video} & CVPR'20 & Event & 56.01 & 90.19 \\
% %Ev-SegNet~\cite{alonso2019ev} & CVPRW'19 & Event & 54.81 & 89.76 \\
% %E2VID~\cite{rebecq2019events} & TRAMI'19 & Event & 48.47 & 85.84 \\
% %\bottomrule
% %\end{tabular}
% %}
% %\caption[Results on DDD17~\cite{Binas2017DDD17ED}]{Comparison of RGB+Event and Event-only semantic segmentation performance on DDD17~\cite{Binas2017DDD17ED}. Methods are grouped by modality and sorted by publication year (newest to oldest). ``$\uparrow$'' means higher is better.}
% %\label{tab:ddd17_results}
% %\end{table}
% 
% %\begin{table}[t!]
% %\centering
% %\caption[Results on DDD17~\cite{Binas2017DDD17ED}]{Comparison of RGB+Event and Event-only semantic segmentation performance on DDD17~\cite{Binas2017DDD17ED}. ``$\uparrow$'' means higher is better.}
% %\resizebox{\textwidth}{!}{ 
% %\begin{tabular}{l|c|c|cc}
% %\toprule
% %\textbf{Method} & \textbf{Venue} & \textbf{Modal} & \textbf{Mean IoU (\%)}~$\uparrow$ & \textbf{Pixel Acc (\%)} \\
% %\midrule
% %KWYAF~\cite{li2025know} & AAAI'25 & Event & 57.69 & - \\
% %ESEG-B~\cite{zhao2025eseg} & AAAI'25 & Event & 57.01 & - \\
% %ESEG-L~\cite{zhao2025eseg} & AAAI'25 & Event & 59.97 & - \\
% %OpenESS~\cite{kong2024openess} & CVPR'24 & Event & 63.00 & - \\
% %ESS-Sup*~\cite{sun2022ess} & ECCV'22 & Event & 61.37 & - \\
% %ESS-Sup~\cite{sun2022ess} & ECCV'22 & Event & 56.67 & - \\
% %ESS~\cite{sun2022ess} & ECCV'22 & Event & 53.09 & - \\
% %EvDistill~\cite{wang2021evdistill} & CVPR'21 & Event & 58.02 & - \\
% %DTL~\cite{wang2021dual} & ICCV'21 & Event & 58.80 & - \\
% %SegFormer~\cite{xie2021segformer} & NIPS'20 & Event & 52.76 & - \\
% %Vid2E~\cite{gehrig2020video} & CVPR'20 & Event & 56.01 & - \\
% %Ev-SegNet~\cite{alonso2019ev} & CVPRW'19 & Event & 54.81 & - \\
% %\midrule
% %Hybrid-Segmentation~\cite{li2025efficient} & AAAI'25 & RGB+Event & 67.31 & - \\
% %HALSIE~\cite{das2024halsie} & WACV'24 & RGB+Event & 60.66 & - \\
% %CMNeXt~\cite{zhang2023delivering} & CVPR'23 & RGB+Event & 72.67 & - \\
% %\midrule
% %Our Model & - & RGB+Event & \textbf{77.85} & - \\
% %\bottomrule
% %\end{tabular}
% %}
% %\label{tab:ddd17_results}
% %\end{table}
% 
% 
% 
% %\begin{table}[htbp]
% %\centering
% %\resizebox{\textwidth}{!}{ 
% %\renewcommand{\arraystretch}{1.2}
% %\setlength{\tabcolsep}{12pt}
% %\begin{tabular}{l|c|c|cc}
% %\toprule
% %\textbf{Method} & \textbf{Venue} & \textbf{Modality} & \textbf{Mean IoU (\%)}~$\uparrow$ & \textbf{Pixel Acc (\%)}~$\uparrow$ \\
% %\midrule
% %Baseline~\cite{cao2024embracing} & ECCV'24 & RGB+Event & 59.51 & 92.25 \\
% %Our Model & - & RGB+Event & \textbf{60.28} & \textbf{92.38} \\
% %\midrule
% %KTBNet~\cite{cai2025keep} & CVPR'25 & RGB+Event & 58.4 & -- \\
% %Any2Seg~\cite{zheng2024learning} & ECCV'24 & RGB+Event & 57.8 & -- \\
% %CMNeXt~\cite{zhang2023delivering} & CVPR'23 & RGB+Event & 57.5 & -- \\
% %CMX~\cite{zhang2023cmx} & TITS'23 & RGB+Event & 56.5 & -- \\
% %HRFuser~\cite{broedermann2023hrfuser} & ITSC'23 & RGB+Event & 42.2 & -- \\
% %TokenFusion~\cite{wang2022multimodal} & CVPR'22 & RGB+Event & 45.6 & -- \\
% %\bottomrule
% %\end{tabular}}
% %\caption[Results on DELIVER-Event~\cite{zhang2023delivering}]{Semantic segmentation results on the DELIVER-Event dataset~\cite{zhang2023delivering}. All experiments are conducted on resized $521 \times 521$ images. ``$\uparrow$'' indicates higher is better.}
% %\label{tab:deliver_event_results}
% %\end{table}
% 
% 
% 
% %\begin{table}[htbp]
% %\centering
% %\renewcommand{\arraystretch}{1.2}
% %\setlength{\tabcolsep}{5pt}
% %\resizebox{\textwidth}{!}{
% %\begin{tabular}{l|c|c|c|c|cc}
% %\toprule
% %\multirow{2}{*}{\textbf{Method}} & 
% %\multirow{2}{*}{\textbf{Venue}} & 
% %\multirow{2}{*}{\textbf{Backbone}} & 
% %\multirow{2}{*}{\textbf{Modality}} & 
% %\multirow{2}{*}{\textbf{Epoch}} & 
% %\multicolumn{1}{c|}{\textbf{UrbanLF-Real}} & 
% %\multicolumn{1}{c}{\textbf{UrbanLF-Syn}} \\
% %\cmidrule(lr){6-6}\cmidrule(l){7-7}
% % & & & & & \textbf{mIoU (\%)}~$\uparrow$ & \textbf{mIoU (\%)}~$\uparrow$ \\
% %\midrule
% %Baseline~\cite{cao2024embracing} & ECCV'24 & MiT-B4 & RGB+LF80 & 60  & 71.25 & 67.05 \\
% %Our Model & - & MiT-B4 & RGB+LF80 & 60  & 79.03 & 77.56 \\
% %Our Model & - & MiT-B4 & RGB+LF80 & 500 & \textbf{83.99} & \textbf{81.91} \\
% %Our Model & - & MiT-B4 & RGB+LF33 & 500 & 83.30 & 81.22 \\
% %Our Model & - & MiT-B4 & RGB+LF8 & 500 & 82.59 & 80.98 \\
% %\midrule
% %OAFuser~\cite{teng2024oafuser} & TAI'24 & MiT-B4 & RGB+LF8  & -   & 82.69 & 81.64 \\
% %CMNeXt~\cite{zhang2023delivering} & CVPR'23 & MiT-B4 & RGB+LF80 & 500 & 83.11 & 81.02 \\
% %CMNeXt~\cite{zhang2023delivering} & CVPR'23 & MiT-B4 & RGB+LF33 & 500 & 82.62 & 80.98 \\
% %CMNeXt~\cite{zhang2023delivering} & CVPR'23 & MiT-B4 & RGB+LF8  & 500 & 83.22 & 80.74 \\
% %OCR-LF~\cite{sheng2022urbanlf} & TCSVT'22 & -- & RGB+LF33 & - & 79.32 & 80.43 \\
% %PSPNet-LF~\cite{zhao2017pyramid} & CVPR'17 & -- & RGB+LF33 & - & 78.10 & 77.88 \\
% %\midrule
% %LFEI-Net~\cite{jia2025harnessing} & ICASSP'25 & -- & LF & - & 83.72 & -- \\
% %LF-IENet++~\cite{cong2024end} & TCSVT'24 & HRNetV2-W48 & LF & - & -- & 80.85 \\
% %LF-EANet~\cite{li2024multi} & ICONIP'24 & MiT-B3 & LF & - & -- & 80.38 \\
% %LFRSNet~\cite{yang2022lfrsnet} & Front. Environ. Sci.'22 & -- & LF & - & 79.98 & 80.87 \\
% %\midrule
% %TMANet~\cite{wang2021temporal} & ICIP' 21 & -- & Video & - & 77.14 & 76.41 \\
% %DAVSS~\cite{zhuang2020video} & TCSVT'20 & -- & Video & - & 75.91 & 74.27 \\
% %\midrule
% %SegFormer~\cite{xie2021segformer} & NeurIPS'21 & -- & RGB & - & 82.20 & 78.53 \\
% %OCR~\cite{yuan2020object} & TCSVT'22 & -- & RGB & - & 78.60 & 79.36 \\
% %PSPNet~\cite{zhao2017pyramid} & CVPR'17 & -- & RGB & - & 76.34 & 75.78 \\
% %\bottomrule
% %\end{tabular}}
% %\caption[Results on UrbanLF~\cite{sheng2022urbanlf}]{Comparison on UrbanLF-real and UrbanLF-syn~\cite{sheng2022urbanlf}. Columns show Mean IoU (mIoU). ``$\uparrow$'' indicates higher is better. ``LF80'', ``LF33'', and ``LF8'' denote using 80, 33, and 8 sub-aperture views as auxiliary modalities.}
% %\label{tab:urbanlf_joint_results}
% %\end{table}
% % \subsection{Use of LLMs}
% % We used ChatGPT (OpenAI) solely for grammar polishing and improving readability in the introduction and related work sections. No content generation, data analysis, or result creation was performed using large language models (LLMs).
% 
% \wrapfinish
